# Supplementary material for: On the detrimental effect of invariances in the likelihood for variational inference
Source: arXiv:2209.07157 source file (2022-10-06)
Supplement: Supplementary file 1 [file scaling.tex]

\subsection{Scaling invariance}
Consider the model 
\begin{align}
\w &\sim p(\w) = \mathcal{N}(\w, \mu, \sigma^2), \\
\y &=  \prod_{k=1}^{K} \w_{k} + \epsilon,
\end{align}
where $\w$ is $K$-dimensional. This model is a product of Gaussian latent variables with a Gaussian likelihood with measurement noise $\epsilon$. 

This model has only 1 degree of freedom. Besides the permutation invariance (ignore here), we have a \emph{scaling invariance} that we could describe as a \emph{translation invariance in log-space}, similarly as above, on the $(K-1)$-dimensional hyperplane with normal vector $(1, 1, \dots, 1)$. 

This invariance can be described by the function 
\begin{align}
 f_{\rep}(\w) = \w \cdot  \mathbf{n}_{\rep} = \exp\left( \log \w + \log \mathbf{n}_{\rep} \right), \\
 f^{-1}_{\rep}(\bv) = \bv / \mathbf{n}_{\rep} = \exp\left( \log \bv - \log \mathbf{n}_{\rep} \right),
\end{align}
where $\log \mathbf{n}_{\rep}$ is any vector on the hyperplane that is perpendicular to its normal vector $(1, 1, \dots, 1)$. 

For example, with $K=2$ components, we have 1 degree of freedom, i.e.\ the line $\mathbf{n}_{\rep}= \rep \cdot (1, -1)$. 
\begin{align}
 f_{\rep}\begin{pmatrix} \w_1 \\ \w_2 \end{pmatrix} 
&= \begin{pmatrix} \w_1 \cdot \rep \\ \w_2 / \rep \end{pmatrix} 
= \begin{pmatrix} \bv_1 \\ \bv_2  \end{pmatrix} 
\\
f^{-1}_{\rep}\begin{pmatrix} \bv_1 \\ \bv_2 \end{pmatrix} 
&= \begin{pmatrix} \bv_1 / \rep \\ \bv_2 \cdot \rep \end{pmatrix} 
= \begin{pmatrix} \w_1 \\ \w_2  \end{pmatrix} 
\end{align}

This transformation is both \emph{bijective} (needs to be shown?) and \emph{volume-preserving}, since the determinant of the derivative is 
\begin{equation}
\left| \frac{d}{d \bv} f_{\rep}^{-1}(\bv) \right| = \frac{1}{\rep} \cdot \rep = 1.
\end{equation}
